# Supplementary material for: EcoTTA: Memory-Efficient Continual Test-time Adaptation via Self-distilled Regularization
Source: arXiv:2303.01904 source file (2023-05-23)
Supplement: Supplementary file 1 [file supple_full_cifar10.tex]

{
\begin{table*}
\centering
\arrayrulecolor{black}
\footnotesize
\vspace{-0.2cm}
\resizebox{.98\textwidth}{!}{
\begin{tabular}{l|l|ccccccccccccccc|c|c|}
\toprule
\textbf{Backbone}                                                              & \textbf{Method}         & Gaus. & Shot & Impu. & Defo. & Glas. & Moti. & Zoom & Snow & Fros. & Fog  & Brig. & Cont. & Elas. & Pixe. & Jpeg &  \textbf{Avg. err {\scriptsize $\downarrow$}} & \textbf{Mem. {\scriptsize $\downarrow$}}   \\
\drule
\multirow{11}{*}{\begin{tabular}[c]{@{}l@{}}WRN40 \\(Aug Mix)\end{tabular}} & Source         & 44.3  & 37.0 & 44.8  & 30.6  & 43.9  & 32.6  & 29.4 & 23.9 & 30.1  & 39.7 & 12.9  & 66.4  & 32.7  & 58.4  & 23.5 & 36.7  & 2                        \\
                                                                            & tBN            & 19.5  & 17.6 & 23.8  & 9.6   & 23.1  & 11.1  & 10.3 & 13.4 & 14.2  & 15.0 & 8.0   & 13.9  & 17.3  & 16.0  & 18.8 & 15.4  & 2                        \\
                                                                            & TENT online    & 16.4  & 13.9 & 19.1  & 8.3   & 19.1  & 9.3   & 8.6  & 10.9 & 11.3  & 12.0 & 6.9   & 11.6  & 14.6  & 12.2  & 15.6 & 12.7  & 188                      \\
                                                                            & TENT continual & 16.4  & 12.2 & 17.1  & 9.1   & 18.7  & 11.4  & 10.4 & 12.7 & 12.4  & 14.8 & 10.1  & 13.0  & 17.0  & 13.3  & 19.0 & 13.3  & 188                      \\
                                                                            & TTT++*         & 19.1  & 16.9 & 22.2  & 9.3   & 21.6  & 10.8  & 9.8  & 12.7 & 13.1  & 14.3 & 7.8   & 13.9  & 15.9  & 14.2  & 17.2 & 14.6  & 391                      \\
                                                                            & SWRNSP         & 15.9  & 13.3 & 18.2  & 8.4   & 18.5  & 9.5   & 8.6  & 11.0 & 10.2  & 11.7 & 7.0   & 8.1   & 14.6  & 11.3  & 15.1 & 12.1  & 400                     \\
                                                                            & NOTE           & 19.6  & 16.4 & 19.9  & 9.4   & 20.3  & 10.3  & 10.1 & 11.6 & 10.6  & 13.3 & 7.9   & 7.7   & 15.4  & 12.0  & 17.3 & 13.4  & 188                      \\
                                                                            & ETAT           & 15.2  & 13.1 & 17.5  & 9.5   & 19.9  & 11.6  & 9.3  & 11.4 & 11.5  & 12.4 & 7.8   & 11.1  & 16.1  & 12.2  & 16.1 & 13.0  & 188                      \\
                                                                            & CoTTA          & 15.6  & 13.6 & 17.3  & 9.8   & 19.0  & 11.0  & 10.2 & 13.5 & 12.6  & 17.4 & 7.8   & 17.3  & 16.2  & 12.9  & 16.0 & 14.0  & 409                     \\
                                                                            & EcoTTA (K=4)     & 16.1  & 13.2 & 18.3  & 8.0   & 18.3  & 9.3   & 8.6  & 10.5 & 10.1  & 12.2 & 6.8   & 11.3  & 14.5  & 11.0  & 14.8 & 12.2  & 80                       \\
                                                                            & EcoTTA (K=5)     & 15.9  & 12.6 & 17.2  & 8.2   & 18.4  & 9.3   & 8.6  & 10.6 & 10.4  & 12.4 & 6.7   & 11.7  & 14.3  & 11.3  & 14.9 & \textbf{12.1}  & 92                       \\ 
\toprule
\multirow{11}{*}{WRN28}                                                     & Source         & 72.3  & 65.7 & 72.9  & 46.9  & 54.3  & 34.8  & 42.0 & 25.1 & 41.3  & 26.0 & 9.3   & 46.7  & 26.6  & 58.5  & 30.3 & 43.5  & 37                       \\
                                                                            & tBN            & 28.6  & 26.8 & 37.0  & 13.2  & 35.4  & 14.4  & 12.6 & 18.0 & 18.2  & 16.0 & 8.6   & 13.3  & 24.0  & 20.3  & 27.8 & 20.9  & 37                       \\
                                                                            & TENT online    & 25.2  & 23.8 & 33.5  & 12.8  & 32.3  & 14.1  & 11.7 & 16.4 & 17.0  & 14.4 & 8.4   & 12.2  & 22.8  & 18.0  & 24.8 & 19.2  & 646                      \\
                                                                            & TENT continual & 25.2  & 20.8 & 29.8  & 14.4  & 31.5  & 15.4  & 14.2 & 18.8 & 17.5  & 17.3 & 10.9  & 14.9  & 23.6  & 20.2  & 25.6 & 20.0  & 646                      \\
                                                                            & TTT++*         & 27.9  & 25.8 & 35.8  & 13.0  & 34.3  & 14.2  & 12.2 & 17.4 & 17.6  & 15.5 & 8.6   & 13.1  & 23.1  & 19.6  & 26.6 & 20.3  & 1405                     \\
                                                                            & SWRNSP         & 24.6  & 20.5 & 29.3  & 12.4  & 31.1  & 13.0  & 11.3 & 15.3 & 14.7  & 11.7 & 7.8   & 9.3   & 21.5  & 15.6  & 20.3 & 17.2  & 1551                    \\
                                                                            & NOTE           & 30.4  & 26.7 & 34.6  & 13.6  & 36.3  & 13.7  & 13.9 & 17.2 & 15.8  & 15.2 & 9.1   & 7.5   & 24.1  & 18.4  & 25.9 & 20.2  & 646                      \\
                                                                            & ETAT           & 23.8  & 18.8 & 27.3  & 13.9  & 29.7  & 16.0  & 13.3 & 18.0 & 16.9  & 15.7 & 10.5  & 12.2  & 22.9  & 17.1  & 23.0 & 18.6  & 646                      \\
                                                                            & CoTTA          & 24.6  & 21.6 & 26.5  & 12.1  & 28.0  & 13.0  & 10.9 & 15.3 & 14.6  & 13.6 & 8.1   & 12.2  & 20.0  & 14.9  & 19.5 & 17.0  & 1697                    \\
                                                                            & EcoTTA (K=4)     & 23.5  & 19.0 & 26.6  & 11.5  & 30.6  & 13.1  & 10.9 & 15.2 & 14.5  & 13.1 & 7.8   & 11.4  & 20.9  & 15.4  & 20.8 & 16.9  & 404                      \\
                                                                            & EcoTTA (K=5)     & 23.8  & 18.7 & 25.7  & 11.5  & 29.8  & 13.3  & 11.3 & 15.3 & 15.0  & 13.0 & 7.9   & 11.3  & 20.2  & 15.1  & 20.5 & \textbf{16.8}  & 471                      \\ 
\toprule
\multirow{10}{*}{Resnet50}                                                  & Source         & 65.6  & 60.7 & 74.4  & 28.9  & 79.9  & 46.0  & 25.7 & 35.0 & 49.4  & 54.7 & 13.0  & 83.2  & 41.2  & 46.7  & 27.7 & 48.8  & 24                       \\
                                                                            & tBN            & 18.0  & 17.2 & 29.3  & 10.7  & 27.2  & 15.5  & 8.9  & 16.7 & 14.6  & 21.0 & 9.3   & 12.7  & 20.9  & 12.4  & 14.8 & 16.6  & 24                       \\
                                                                            & TENT online    & 16.6  & 15.7 & 25.7  & 10.0  & 24.8  & 13.8  & 8.3  & 14.9 & 13.8  & 17.6 & 8.7   & 10.0  & 19.1  & 11.5  & 13.8 & 15.0  & 925                      \\
                                                                            & TENT continual & 16.6  & 14.4 & 22.9  & 10.4  & 22.6  & 13.4  & 10.3 & 15.8 & 14.6  & 18.0 & 10.5  & 11.7  & 18.4  & 13.1  & 15.3 & 15.2  & 925                      \\
                                                                            & TTT++          & 18.2  & 16.9 & 28.7  & 10.5  & 26.5  & 14.5  & 8.9  & 16.5 & 14.5  & 20.9 & 9.0   & 9.0   & 20.4  & 12.3  & 14.7 & 16.1  & 1877                     \\
                                                                            & SWRNSP         & 17.3  & 16.1 & 26.1  & 10.6  & 25.6  & 14.1  & 8.7  & 15.6 & 13.6  & 18.6 & 8.8   & 10.0  & 19.3  & 12.0  & 14.2 & 15.4  & 1971                    \\
                                                                            & ETAT           & 17.2  & 14.9 & 23.6  & 10.2  & 23.3  & 13.2  & 8.5  & 14.0 & 12.5  & 16.6 & 8.6   & 9.4   & 17.2  & 11.0  & 12.7 & 14.2  & 925                      \\
                                                                            & CoTTA          & 16.2  & 15.0 & 21.2  & 10.4  & 22.8  & 13.9  & 8.4  & 15.1 & 12.9  & 19.8 & 8.6   & 11.3  & 17.5  & 10.5  & 12.2 & 14.4  & 2066                    \\
                                                                            & EcoTTA (K=4)     & 16.5  & 14.5 & 24.3  & 9.7   & 23.7  & 13.3  & 8.8  & 14.7 & 12.9  & 17.0 & 9.1   & 9.4   & 17.6  & 11.4  & 13.1 & 14.4  & 296                      \\
                                                                            & EcoTTA (K=5)     & 16.6  & 14.4 & 23.6  & 9.8   & 23.4  & 12.7  & 8.6  & 14.5 & 12.6  & 16.6 & 8.7   & 9.0   & 17.0  & 11.3  & 12.6 & \textbf{14.1}  & 498                      \\
\toprule
\end{tabular}}
\footnotesize
\vspace{-0.3cm}
\caption{Comparison of error rate ($\%$) on \textbf{CIFAR-10-C} with severity level 5}
\arrayrulecolor{black}
\end{table*}}
