# Supplementary material for: EcoTTA: Memory-Efficient Continual Test-time Adaptation via Self-distilled Regularization
Source: arXiv:2303.01904 source file (2023-05-23)
Supplement: Supplementary file 2 [file supple_full_cifar100.tex]

{
\begin{table*}
\centering
\arrayrulecolor{black}
\resizebox{.98\textwidth}{!}{
\begin{tabular}{l|l|ccccccccccccccc|c|c|} 
\toprule
\textbf{Backbone}                                                                        & \textbf{Method}         & Gaus. & Shot & Impu. & Defo. & Glas. & Moti. & Zoom & Snow & Fros. & Fog  & Brig. & Cont. & Elas. & Pixe. & Jpeg &  \textbf{Avg. err {\scriptsize $\downarrow$}} & \textbf{Mem. {\scriptsize $\downarrow$}}     \\ 
\drule
\multirow{11}{*}{\begin{tabular}[c]{@{}l@{}}WRN40 \\(Aug Mix)\end{tabular}} & Source         & 80.1  & 77.0 & 76.4  & 59.9  & 77.6  & 64.2  & 59.3 & 64.8 & 71.3  & 78.3 & 48.1  & 83.4  & 65.8  & 80.4  & 59.2 & 69.7  & 2                        \\
                                                                            & tBN            & 45.9  & 45.6 & 48.2  & 33.6  & 47.9  & 34.5  & 34.1 & 40.3 & 40.4  & 47.1 & 31.7  & 39.7  & 42.7  & 39.2  & 45.6 & 41.1  & 2                        \\
                                                                            & TENT online    & 41.2  & 40.6 & 42.2  & 30.9  & 43.4  & 31.8  & 30.6 & 35.3 & 36.2  & 40.1 & 28.5  & 35.5  & 39.1  & 33.9  & 41.7 & 36.7  & 188                      \\
                                                                            & TENT continual & 41.2  & 38.2 & 41.0  & 32.9  & 43.9  & 34.9  & 33.2 & 37.7 & 37.2  & 41.5 & 33.2  & 37.2  & 41.1  & 35.9  & 45.1 & 38.3  & 188                      \\
                                                                            & TTT++*         & 46.0  & 45.4 & 48.2  & 33.5  & 47.7  & 34.4  & 33.8 & 39.9 & 40.2  & 47.1 & 31.8  & 39.7  & 42.5  & 38.9  & 45.5 & 41.0  & 391                      \\
                                                                            & SWRNSP         & 42.4  & 40.9 & 42.7  & 30.6  & 43.9  & 31.7  & 31.3 & 36.1 & 36.2  & 41.5 & 28.7  & 34.1  & 39.2  & 33.6  & 41.3 & 36.6  & 400                     \\
                                                                            & NOTE           & 50.9  & 47.4 & 49.0  & 37.3  & 49.6  & 37.3  & 37.0 & 41.3 & 39.9  & 47.0 & 35.2  & 34.7  & 45.2  & 40.9  & 49.9 & 42.8  & 188                      \\
                                                                            & ETAT           & 41.6  & 39.9 & 41.2  & 31.7  & 44.0  & 32.4  & 31.9 & 36.2 & 36.8  & 39.7 & 29.1  & 34.4  & 39.9  & 34.2  & 42.2 & 37.1  & 188                      \\
                                                                            & CoTTA          & 43.5  & 41.7 & 43.7  & 32.2  & 43.7  & 32.8  & 32.2 & 38.5 & 37.6  & 45.9 & 29.0  & 38.1  & 39.2  & 33.8  & 39.4 & 38.1  & 409                     \\
                                                                            & EcoTTA (K=4)     & 42.7  & 39.6 & 42.4  & 31.4  & 42.9  & 31.9  & 30.8 & 35.1 & 34.8  & 40.7 & 28.1  & 35.0  & 37.5  & 32.1  & 40.5 & 36.4  & 80                       \\
                                                                            & EcoTTA (K=5)     & 41.8  & 39.0 & 41.9  & 31.2  & 42.7  & 32.5  & 31.0 & 35.0 & 35.0  & 39.9 & 28.8  & 34.5  & 37.5  & 32.8  & 40.5 & \textbf{36.3}  & 92                       \\ 
\toprule
\multirow{10}{*}{Resnet50}                                                  & Source         & 84.7  & 83.5 & 93.3  & 59.6  & 92.5  & 71.9  & 54.8 & 66.6 & 77.6  & 81.8 & 44.3  & 91.2  & 72.2  & 76.6  & 56.5 & 73.8  & 24                       \\
                                                                            & tBN            & 48.1  & 46.7 & 60.6  & 35.1  & 58.0  & 41.8  & 33.2 & 47.3 & 43.5  & 54.9 & 33.5  & 35.3  & 49.8  & 38.4  & 40.8 & 44.5  & 24                       \\
                                                                            & TENT online    & 44.1  & 42.7 & 53.9  & 32.6  & 52.0  & 37.5  & 30.5 & 43.4 & 40.2  & 45.7 & 30.4  & 31.4  & 45.1  & 35.0  & 37.6 & 40.1  & 926                     \\
                                                                            & TENT continual & 44.0  & 40.1 & 49.9  & 34.7  & 50.6  & 40.0  & 33.6 & 47.0 & 45.7  & 53.4 & 42.5  & 46.2  & 56.1  & 51.2  & 53.3 & 45.9  & 926                     \\
                                                                            & TTT++          & 48.1  & 46.5 & 60.8  & 35.1  & 57.8  & 41.6  & 32.9 & 46.8 & 43.3  & 55.0 & 33.3  & 34.0  & 50.0  & 38.1  & 40.6 & 44.2  & 1876                    \\
                                                                            & SWRNSP         & 48.3  & 46.5 & 60.5  & 35.1  & 57.9  & 41.7  & 32.9 & 47.1 & 43.5  & 54.7 & 33.5  & 35.1  & 49.9  & 38.3  & 40.7 & 44.1  & 1970                   \\
                                                                            & ETAT           & 44.8  & 41.9 & 52.6  & 33.0  & 51.1  & 37.8  & 30.3 & 43.0 & 40.1  & 45.1 & 30.1  & 31.8  & 45.2  & 35.2  & 37.4 & 39.9  & 926                     \\
                                                                            & CoTTA          & 43.6  & 42.8 & 50.4  & 34.2  & 51.6  & 39.2  & 31.4 & 43.4 & 39.6  & 47.4 & 31.3  & 32.2  & 43.4  & 35.8  & 36.7 & 40.2  & 2064                   \\
                                                                            & EcoTTA (K=4)     & 46.4  & 40.7 & 50.2  & 31.1  & 48.7  & 35.2  & 29.4 & 40.8 & 39.6  & 45.3 & 30.8  & 35.8  & 44.1  & 36.4  & 38.7 & 39.5  & 296                     \\
                                                                            & EcoTTA (K=5)     & 46.4  & 41.0 & 49.1  & 31.3  & 48.9  & 35.6  & 29.6 & 41.2 & 38.5  & 44.4 & 30.7  & 35.1  & 43.5  & 36.2  & 38.8 & \textbf{39.3}  & 498                     \\
\toprule
\end{tabular}}
\footnotesize
\vspace{-0.3cm}
\caption{Comparison of error rate ($\%$) on \textbf{CIFAR-100-C} with severity level 5}
\arrayrulecolor{black}
\end{table*}}
